# Supplementary material for: Investigation of Electroweak Production of the Top Quark at the LHC
Source: arXiv:0804.3706 source file (2008-04-23)
Supplement: Supplementary file 1 [file Appendix.tex]

% will indicate texshop to compile root file
%%!TEX root = ../Main.tex

\chapter{Appendix}

\section{Definitions}

%The beam direction defines the z-axis, and the x-yplane is the planetransverse to the beam direction. Thepositive xaxisisdefinedaspointingfromtheinteractionpointtothecentreofthe LHCring, andthepositivey-axisispointingupwards. Theazimuthal angle?ismeasured aroundthebeamaxis,andthepolarangle?istheanglefromthebeamaxis.Thepseudorapidity isdefinedas . Thetransversemomentump TandthetransverseenergyET, as wellasthemissingtransverseenergyE Tmissandothertransversevariables,aredefinedinthex- yplaneunlessstatedotherwise.ThedistanceÆRinthepseudorapidity-azimuthalanglespaceis defined as . Trajectoriesofchargedparticlescanbedescribedbyfivehelixparametersinanideal uniform magneticfield. ThefollowinghelixparametrisationisusedinATLAS, withallquantitiesmeas- uredat thepoint of closest approachtothenominal beamaxisx=0, y=0. Parametersinx-y plane are: 1/p T Reciprocal of the transverse momentum with respect to the beam-axis. ? Azimuthal angle, where tan??py/px. d 0 Transverseimpact parameter, definedas thetransversedistancetothe beamaxisatthepointofclosestapproach; signedaccordingtotherecon- structed angular momentum of the track about the axis. Parameters in theR-z plane are: cot? Cotangent of the polar angle, where cot??p z/pT; z 0 Longitudinalimpactparameter,definedasthezpositionofthetrackatthe point of closest approach. ? ? 2Ö( )tanlnÐ= ÆR Æ2? + Æ2?=

\et
\pt
\deltaR

\section{Units and Constants}
\begin{table}[htdp]
\begin{center}
\begin{tabular}{|l|l|c|}
\hline
Quality & Symbol & Value\\
\hline \hline
Cross section & $\sigma$  & $1 b = 1\times 10^{-24} cm^{2}$\\
\hline
\end{tabular}
\caption{An useful conversion table for reference}
\label{UnitsConstants}
\end{center}
\end{table}
